# Supplementary material for: The role of fast ions in stabilising the ion temperature gradient mode
Source: arXiv:1712.03587 source file (2017-12-10)
Supplement: Supplementary file 1 [file B.tex]

\documentclass[class=book,float=false, crop=false,11pt, a4paper]{standalone}
\usepackage{./StyFiles/packages} % Extra 
\begin{document}
\chapter{Derivation of the Grad-Shafranov equation}\label{sec:App:B}
Here we outline the main steps in the derivation of the Grad-Shafranov Eq.~\eqref{eq:App:Geometry:GS}.

The tokamak is a toroidal systems with toroidal symmetry so we write the gradient operator $\nabla$ as
\eq{
\nabla \cdot \vecB = \frac{1}{R}\dpd{}{R}(RB_R) + \dpd{B_Z}{Z},
}
where $\vecB = \hat R B_R + \hat \phi B_{\phi} + \hat Z B_Z$ is the magnetic field.  Here $\hat R,\hat \phi,\hat Z$ denote the unit vector in the radial, azimuthal and the vertical $Z$ coordinates respectively. By virtue of Eq.~\eqref{eq:Geometry:MHD3} we can write the field as $\vecB = \nabla \times \vecA$ where $\vecA$ is the well known vector potential.
Evaluating the components gives
\eqre{
\label{eq:Geometry:cross}
\nabla \times \vecA = -\hat R \dpd{A_{\phi}}{Z}  + \hat \phi \left(\dpd{A_R}{Z}-\dpd{A_Z}{R}\right) + \hat Z \frac{1}{R}\dpd{}{R}(RA_{\phi}).
}

It is convenient to write $\Psi =  RA_{\phi}$ such that

\eqre{
\label{eq:PreSim:Geometry:Bfield}
\vecB = \nabla \phi \times \nabla \Psi + \nabla \phi \frac{B_{\phi}}{R},
}
were $\nabla \phi = \hat \phi/R$. 
If we evaluate the poloidal flux of the magnetic field going through a surface $\Omega$ in the toroidal plane, radially limited by $R = R_1$ and $R = R_2$ with $R_2 > R_1$, we see that
\eq{
\int_{\Omega_p} \vecB \text{d}\vecS = 2\pi\int_{R_1}^{R_2} R \vecB_Z \text{d}R = \left[Eq.~\eqref{eq:Geometry:cross} \right] = 2\pi \int_{R_1}^{R_2} \frac{1}{R}\dpd{}{R}(RA_{\phi})R\text{d}R = \Psi(R_2) - \Psi(R_1).
}
Henceforth we will therefor refer to $\Psi$ as the poloidal flux. Using Eq.~\eqref{eq:PreSim:Geometry:Bfield} in Eq.~\eqref{eq:Geometry:MHD2} and evaluating the cross product terms explicitly we get
\eq{
\vecJ = \nabla \phi \underbrace{\left[\dpd[2]{}{Z}\Psi - \frac{1}{R}\dpd{\Psi}{R} + \dpd[2]{}{R}\Psi\right]}_{\Delta^* \Psi} + \nabla \times (\hat \phi B_{\phi}),
}
where we defined the operator $\Delta^*$. The second cross product term may be written as
\eq{
\nabla \times (\hat \phi B_{\phi}) = B_{\phi}\nabla \times \hat \phi + \nabla B_{\phi} \times \hat \phi = \frac{B_{\phi}}{R}\hat Z + \nabla B_{\phi} \times \hat \phi,
}
since $\nabla \times \hat \phi = \hat Z/R$.  We introduce $f = RB_\phi$ such that the full expression for the current becomes
\eq{
\vecJ = \nabla \phi \Delta^*\Psi + \nabla f \times \nabla \phi.
}
Now, taking the scalar product of $\vecB$ with Eq.~\eqref{eq:Geometry:MHD1} we obtain
\eqre{
\label{eq:PreSim:Geometry:pFunPsi}
\vecB \cdot \nabla p = \vecB \cdot \left(\vecJ \times \vecB\right) =  0 \implies \\
\nabla \Psi \parallel \nabla p$, \qquad $p \equiv p(\Psi),
}
the pressure is a function of the poloidal flux $\Psi$ only. Similarly we get also $f \equiv f(\Psi)$. The gradients of both quantities, $\nabla p$ and $\nabla f$ can therefore be computed with respect to $\Psi$ only. As we may note Eq.~\eqref{eq:PreSim:Geometry:pFunPsi} implies that the magnetic field lies on constant pressure surfaces~\cite{ref:Freidberg2007}. Same holds for the current $\vecJ$. Since $p = p(\Psi)$ we use the poloidal flux $\Psi$ to label these surfaces, which are more commonly known as \textit{flux surfaces}.

Expanding the toroidal force balance in Eq.~\eqref{eq:Geometry:MHD1} we get
\eq{
\nabla p = \dod{p}{\Psi}\nabla \Psi = \left (\nabla \phi \Delta^*\Psi + \nabla f \times \nabla \phi\right) \times \left(\nabla \phi \times \nabla \psi + f\nabla\phi\right) = -\frac{\Delta^*\Psi\nabla \phi}{R^2}-f\dod{f}{\Phi}\frac{\nabla{\phi}}{R^2}.
}
Rearranging the terms finally gives the nonlinear second order differential equation we where looking for
\eqre{
\label{eq:App:Geometry:GS}
\Delta^* \Psi = -\mu_0r^2p'-ff',
}
known as the Grad-Shafranov (G-S) equation~\cite{ref:Grad1958}. In Eq.~\eqref{eq:App:Geometry:GS} the primed quantities denote $f' = \dod{f}{\Psi}$ and equivalently for $p'$. 

%defines a magnetic equi
%Given the effects of fast ions on the pressure gradient $p'$, the toroidal 
%This is a nonlinear second order differential equation. Finding a solution requires us to specify $ff'$, $p'$ and the boundary flux surface $\Psi_0$. The solution then provides us with the flux surfaces for all radii $r$ which defines an equilibrium.

% The shape of theses surfaces is what characterises a toroidal MHD equilibrium.

%Examples of flux surfaces is given in Fig.~\ref{fig:PreSim:Geometry:FluxEx} 

%integrated over some poloidal cross section $\Omega$. Since the magnetic field lies on constant pressure surfaces the above expression can be seen as a function of the pressure. For each value of $p$ we get a value of $\Psi_p$. From now on we therefore label $\psi_p$ or simply $\psi$ as a flux surface. 

 % Let us introduce the streaming function $\Psi = RA_{\phi}$ where $A_{\phi}$ is the poloidal component of the magnetic potential. We can then represent the poloidal component of the magnetic field as $\vecB_p = \frac{1}{R}\nabla\psi\times \hat e_{phi}$, where $\hat e_{phi}$ is the unit vector in the poloidal direction.
 
 %From force balance we directly get $\vecB \cdot \nabla p = 0$ which tells us that the magnetic field lies on a constant pressure surfaces known as flux surfaces. 

\end{document}
